# Supplementary material for: HARQ and AMC: Friends or Foes?
Source: arXiv:1606.05177 source file (2016-06-16)
Supplement: Supplementary file 1 [file Appendix.tex]

 \section{Proof of  \theref{Thm22}}\label{sec.appendix.E}

Our objective is to derive a sufficient conditions under which $\displaystyle{\eta=\frac{R(1-f_{K})}{1+\sum_{k=1}^{K} f_{k}}}$ is increasing with $K$, where, for brevity, the relationship on $l$ and $\SNR$ is removed from \eqref{eta.harq.slow.l}.

\begin{align}\label{eta.harq.appendix}
\eta_{K}&\leq\eta_{K+1}\\
\frac{R\big(1-f_{K}\big)}{1+\sum_{k=1}^{K-1} f_{k}} &\le\frac{R\big(1-f_{K+1}\big)}{1+\sum_{k=1}^{K} f_{k}}\\
f_{K+1}\big(1 + \sum_{k=1}^{K-1}  f_{k}\big) &\le f_{K}\sum_{k=1}^{K}  f_{k}\\ 
\label{final.cond}
\sum_{k=1}^{K} f_{K+1} f_{k-1} &\le \sum_{k=1}^{K} f_{K} f_{k}.
\end{align}

Obviously, \eqref{final.cond} is sufficient and necessary condition for the throughput be increasing with $K$. To remove the dependence on the sum we strengthen \eqref{final.cond} imposing inequality on each term which yields sufficient (not necessary) condition
\begin{align}\label{}
f_{K+1} f_{k-1}\le f_{K} f_{k}\quad  \forall k\le K,
\end{align}
that is
\begin{align}\label{eq:condition1}
\frac{f_{K+1}}{f_{K}} \le \frac{f_{k}}{f_{k-1} }\quad  \forall k\le K .
\end{align}

Since \eqref{eq:condition1} must  hold $\forall K \ge 1$, we obtain \eqref{fk.cond.sup}. Any strict inequality in \eqref{eq:condition1}  will make the inequality in \eqref{eta.harq.appendix} strict as well. This terminates the proof.
